# Supplementary material for: Terahertz magneto-optical response in ferromagnetic Fe-Co-Al alloys
Source: arXiv:2202.05997 source file (2024-04-24)
Supplement: Supplementary file 1 [file si.pdf]

# Supplemental Information for “Spin-orbit driven terahertz optical response in ferromagnetic Fe-Co-Al alloys”

Ming Lei<sup>1</sup> and Sinisa Coh<sup>2</sup>

<sup>1</sup>*Chemical and Environmental Engineering, University of California Riverside, California 92521, USA*

<sup>2</sup>*Materials Science and Mechanical Engineering, University of California Riverside, California 92521, USA*

(Dated: February 11, 2022)

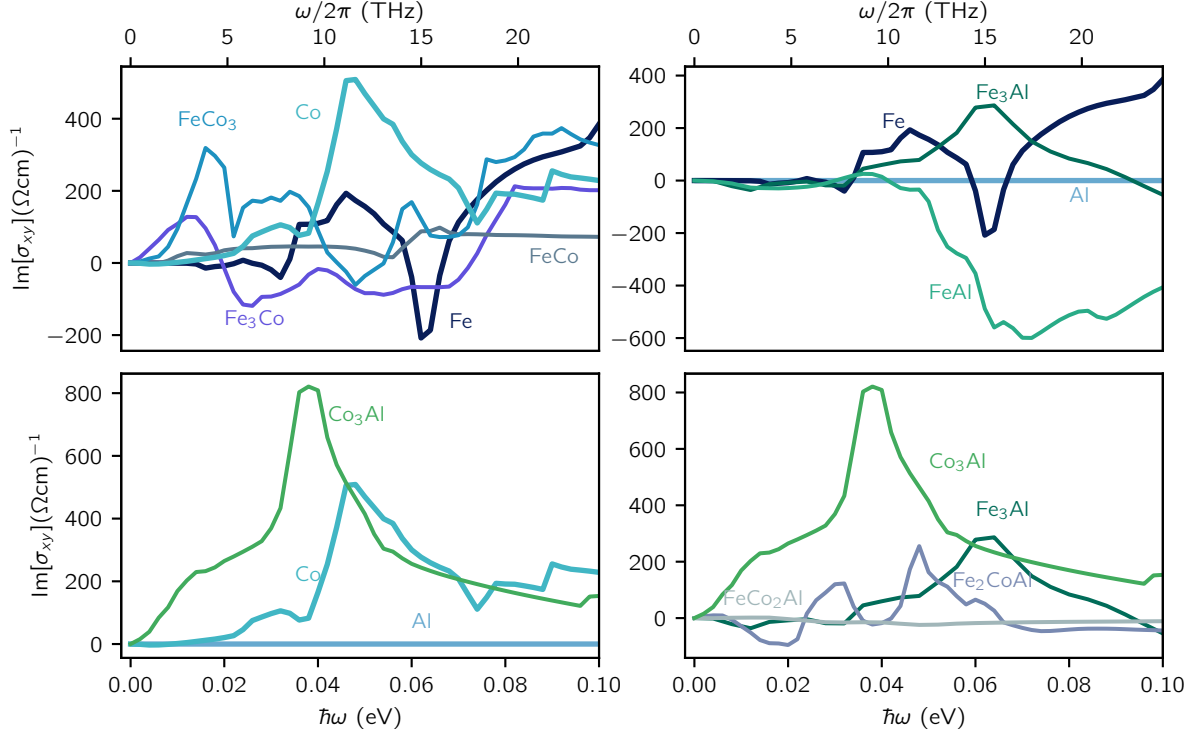

FIG. 1. Calculated imaginary part of  $\sigma_{xy}$  for Fe-Co-Al metals and alloys as a function of frequency  $\omega$ . All conventions are the same as in the main text.

<sup>1</sup> M. Cazzaniga, L. Caramella, N. Manini, and G. Onida, *Phys. Rev. B* **82**, 035104 (2010).

<sup>2</sup> N. D. Mermin, *Phys. Rev. B* **1**, 2362 (1970).

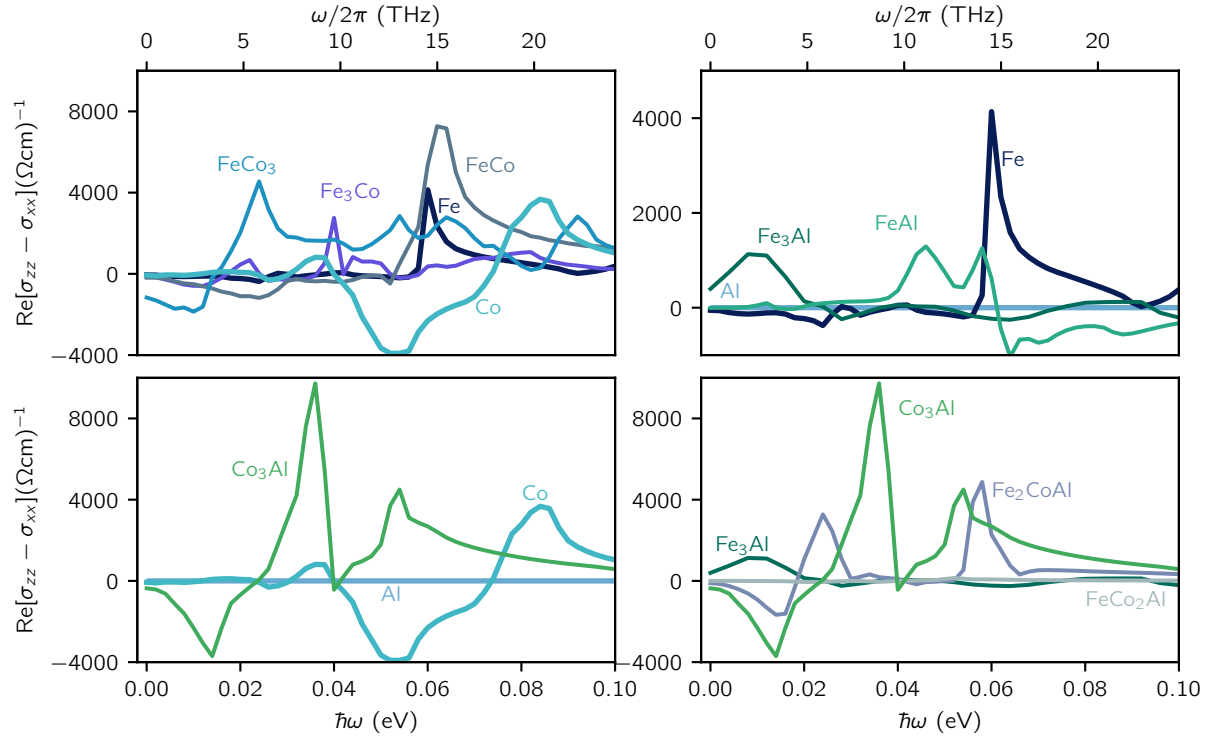

FIG. 2. Calculated real part of  $\sigma_{zz}-\sigma_{xx}$  for Fe-Co-Al metals and alloys as a function of frequency  $\omega$ . All conventions are the same as in the main text

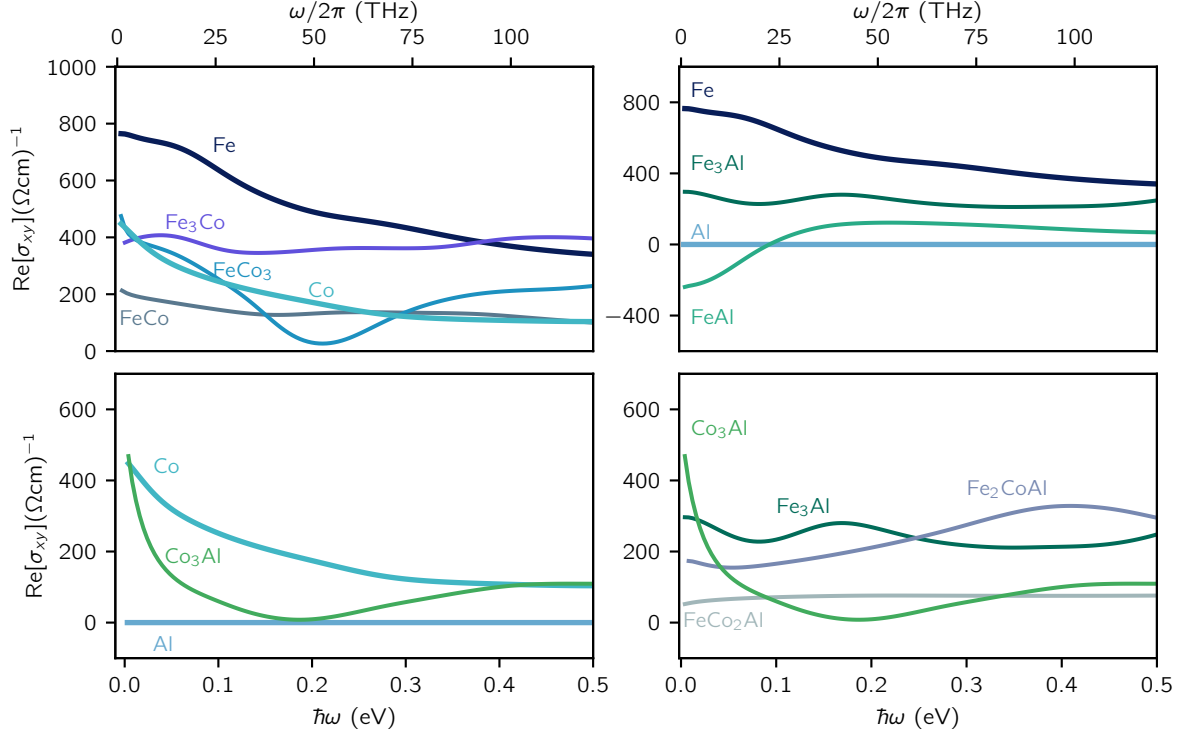

FIG. 3. Calculated real part of  $\sigma_{xy}$  for Fe-Co-Al metals and alloys with a simplified model that incorporates electron lifetime. The range of frequencies in this plot is larger than that in other parts of the manuscript. Frequencies go from 0 to 125 THz. We use model from Ref. 1 to approximately incorporate effect of electron lifetime into our calculation, as it is well known<sup>2</sup> that simply using  $\omega + i\delta$  for finite  $\delta$  leads to the wrong dependence of conductivity in metals at low frequencies. Following the model from Ref. 1 we replace  $\lim_{\delta \rightarrow 0} (\dots \omega + i\delta/2)^{-1}$  in our Kubo formula in the main text with  $\sqrt{\omega(\omega + i\delta)}$  and we use a finite value,  $\delta = 0.2$  eV that is close to the average inverse electron lifetime in Fe-Co-Al alloys.
